# Supplementary material for: A Survey on Hypergraph Neural Networks: An In-Depth and Step-By-Step Guide
Source: arXiv:2404.01039 source file (2024-07-25)
Supplement: Supplementary file 1 [file 999Appendix.tex]

% In this appendix, we compare the four design components of HNNs (Sec.~\ref{sec:encoding} and Sec.~\ref{sec:training}) with those of graph neural networks (GNN).

% \smallsection{Design features.}
% \red{GNNs also require node and/or edge features to represent pairwise graphs.
% Most of the techniques described in Sec.~\ref{subsec:externalfeatures} and Sec.~\ref{subsec:identityfeatures} have their direct counterparts in pairwise graphs~\citep{yang2016revisiting, yoo2022accurate}.
% However, typical structural features for GNNs~\cite{grover2016node2vec, wang2022equivariant} do not focus on HOIs.}
% %, while those for HNNs aim to capture HOIs (Sec.~\ref{subsec:structuralfeatures}).


% \smallsection{Express graphs.}
% \red{In GNNs, the graph structure is typically expressed with an adjacency matrix. 
% Due to its more straightforward nature, a different transformation of the graph structure is not typically done in GNNs.
% Also, recall that the reductive transformation (Sec.~\ref{subsec:clique_expansion}) converts a hypergraph into a pairwise graph, making the standard GNNs to be readily applicable to the transformed hypergraph.
% In contrast, the non-reductive transformation (Sec.~\ref{subsec:star_expansion}) returns (1) graphs of multiple node types or (2) tensors.
% As a result, typical GNNs, such as GCN~\cite{kipf2016semi} and GAT~\citep{velivckovic2017graph}, are not suitable for these transformed hypergraphs.}

% \smallsection{Pass messages.}
% \red{GNNs also utilize neural message passing functions to aggregate information from other nodes~\cite{gilmer2017neural, lee2023towards, liang2024sign}.
% Several HNNs directly utilize GNN's message passing technique on clique-expanded graphs~\cite{feng2019hypergraph, tang2024hypergraph}.
% However, to learn hyperedge representations or hyperedge-dependent node representations, it may be more suitable to use techniques specifically designed for such purposes (Sec.~\ref{subsec:whom2whom} and Sec.~\ref{subsec:aggregation}).
% This is because, with few exceptions~\cite{jo2021edge}, GNNs typically perform message passing directly between nodes, without explicitly considering (hyper)edge representations.
% } %, rampavsek2022recipe

% \smallsection{Design objective (interaction classification).}
% \red{Link prediction on pairwise graphs is a counterpart of the HOI classification task, and various GNN architectures have been developed to tackle the link prediction task~\cite{zhu2021neural, zhang2018link}.
% While both (pairwise) link prediction and HOI classification aim to classify positive and negative interactions, the space of possible negative interactions significantly differs.
% In pairwise graphs, each edge consists of two nodes, and therefore, the size of the space is $O(\vert \mathcal{V}\vert^{2})$.
% However in hypergraphs, since a hyperedge can contain an arbitrary number of nodes, the size of the space is $O(2^{\vert \mathcal{V}\vert})$, which is much greater than that in pairwise graphs.
% Thus, finding representative negative HOIs, or hyperedges, is considered much more challenging than finding representative negative pairwise edges~\cite{hwang2022ahp}.}

% \smallsection{Design objective (contrastive learning)}
% \red{GNNs are also widely trained with CL~\cite{velivckovic2018deep, qiu2020gcc}.
% The overall training scheme is similar to that for HNNs, generating multiple views and contrasting their representations.
% However, CL for GNNs typically focuses on node-level contrastive losses~\cite{velivckovic2018deep} and graph-level contrastive losses~\cite{qiu2020gcc}.}

% \smallsection{Design objective (interaction generation)}
% \red{Various GNNs also target to generate ground-truth pairwise interactions~\cite{kipf2016variational} or latent pairwise interactions~\cite{fatemi2021slaps}.
% However, such techniques developed for pairwise graphs cannot be directly applied to generate HOIs.
% Specifically, in a pairwise graph, the inner product of two node embeddings is widely utilized to model the likelihood of the corresponding two nodes being joined by an edge~\cite{kipf2016variational, fatemi2021slaps}.
% However, since a hyperedge can connect any number of nodes, the likelihood of a certain HOI cannot be modeled via the inner product operation.
% Thus, specialized generation techniques (Sec.~\ref{subsec:gengroundtruthhoi} and Sec.~\ref{subsec:genlatenthoi}) are necessary to generate HOIs.}
